# Supplementary material for: Peer Feedback and Forecast Revision
Source: arXiv:2509.01264 ancillary file (2026-11-23)
Supplement: Supplementary file 1 [file SL_expPrec_slides.pdf]

# Social Learning from Experts with Uncertain Precision

---

Georgy Lukyanov

Toulouse School of Economics  
georgy.lukyanov@tse-fr.eu

1. Motivation and setup
2. Binary baseline: one-sided distortion & closed-form mixing
3. Aggregation and design: additive log-likelihood; proper scoring  $\Rightarrow$  KL
4. Gaussian extension: mimicry coefficient and linear filtering
5. Correlated signals: GLS weighting
6. Estimation & quick empirical handles
7. Applications & takeaways

# Motivation

---

# What are we learning from expert panels?

- Not just the *state of the world* — also *who is actually skilled*.
- Experts care about reputation; true precision is unknown.
- Observer must: (i) learn the persistent truth; (ii) rank experts by precision.
- Settings: medical guidelines, monetary policy committees, forecasting platforms, climate assessments.

# What we do

- Model repeated public opinions with heterogeneous (unknown) precision and reputational incentives.
- Characterize a simple reporting equilibrium:
  - High-precision: truthful; Low-precision: *one-sided* shading around the public prior.
- Aggregation is additive in log-likelihood ratios; reputations update by Bayes.
- Light-touch design (evaluation windows or small convex costs) restores strict informativeness and consistency.

## Binary baseline: results

---

# Static equilibrium at a fixed public prior

- Single-crossing: when high types are truthful, the low type's incentive to shade is one-sided.
- Unique closed-form mixing probabilities:
  - Below a balanced prior: only “favorable” reports are shaded; above: only “unfavorable.”
  - Mixing probabilities depend on the public prior and the precision gap, not on the fraction of high types.
- Dynamics: reputations polarize; aggregation converges toward reputation-weighted voting.

# Mixing probabilities

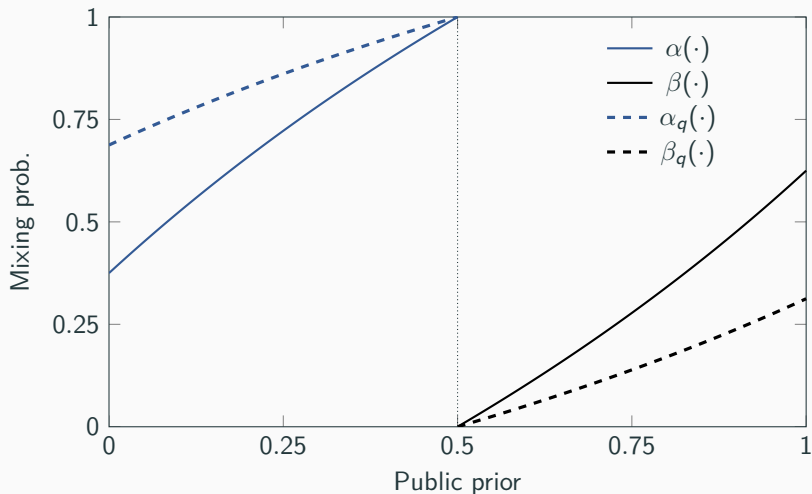

Dashed curves implement an illustrative evaluation density  $q$ :

$$\alpha_q = (1 - q)\alpha + q, \beta_q = (1 - q)\beta.$$



# Aggregation and design

---

# Aggregation and reputations (high-level)

- Aggregation adds up per-expert log-likelihood increments; reputations update by Bayes.
- Independence across experts is the baseline; common shocks  $\Rightarrow$  GLS.
- Light-touch design:
  - Evaluation windows scored by strictly proper rules;
  - or a small convex deviation cost.
- Either device ensures per-evaluation information is *strictly* positive on average.

## Proper scoring $\Rightarrow$ Kullback–Leibler (the key identity)

### Log score (strictly proper)

Expected score advantage of truth at evaluation dates equals KL divergence:

$$\mathbb{E}_{P_\theta} [\log p_\theta(Y)] - \mathbb{E}_{P_\theta} [\log q(Y)] = D_{\text{KL}}(P_\theta \| Q) > 0 \text{ if } Q \neq P_\theta.$$

- Implies per-evaluation log-likelihood increments have positive mean.
- With positive evaluation density, cumulative information diverges  $\Rightarrow$  consistency.

## Gaussian extension

---

## Gaussian extension: what changes?

- Reports are continuous; filtering is linear.
- Low type's one-shot best reply is a *mimicry coefficient*: he shrinks toward the public prior less than the high type.
- Evaluation dates still induce truth by proper scoring; small convex deviation costs move the low type toward truth off evaluation dates.

## Estimation and quick diagnostics

---

## Simple diagnostics on evaluation dates

- Probability reports: logistic calibration (GLM) for intercept and responsiveness.
- Continuous reports: two-line MLE for bias and precision from scored residuals.
- Reliability diagrams & leaderboard dynamics provide quick empirical touchpoints.

## **Applications & takeaways**

---



# Applications and design implications

- Medical/science panels, monetary policy committees, forecasting platforms, climate assessments.
- Design levers:
  - Announce evaluation windows; use proper scoring.
  - Incorporate small convex costs for deviations from signals (soft discipline).
  - Handle common shocks by GLS weighting.

# Takeaways

1. Unknown precision with reputation yields *one-sided* distortion, closed-form mixing.
2. Additive log-likelihood aggregation; reputations polarize; identification under design.
3. Gaussian analogue with mimicry; correlation slows learning but not cross weights under equal loading.
4. Lightweight tools (evaluation windows; small convex costs) restore strict informativeness.

**Questions?**

## Static mixing: closed forms (for reference)

Let  $A(p; \lambda) = (1 - \lambda) + (2\lambda - 1)p$  with  $1/2 \leq p_L < p_H < 1$ .

- Below a balanced prior:  $\alpha(\lambda) = \frac{A(p_H; \lambda)}{A(p_L; \lambda)}$  on  $\lambda < 1/2$ .
- Above:  $\beta(\lambda) = \frac{A(p_H; \lambda) - A(p_L; \lambda)}{1 - A(p_L; \lambda)}$  on  $\lambda > 1/2$ .

## Existence & uniqueness (sketch)

Monotone indifference map  $\Rightarrow$  unique one-sided mix at each prior; selection via off-path beliefs (D1-consistent).

## Design: proper scoring implies KL

Strict propriety  $\Leftrightarrow$  convex entropy; expected score gap equals a Bregman divergence. For log score it is KL; with positive evaluation density, cumulative information diverges almost surely.

# Gaussian mimicry

If the high type is truthful, the low type's best-response shrinkage is

$$a^{\text{mim}} = \sqrt{\frac{V + \sigma_H^2}{V + \sigma_L^2}} \in (0, 1),$$

equalizing predictive variances across types. Evaluation dates set  $a^* = 1$ ; small convex costs move  $a^*$  toward 1 off evaluation dates.

## Correlation: GLS weights (statement)

Under a common shock with  $\Sigma = D + \tau^2 \mathbf{1}\mathbf{1}^\top$ , the efficient increment uses

$$w \propto \Sigma^{-1} \mathbf{1}, \quad \Sigma^{-1} = D^{-1} - D^{-1} \mathbf{1} \frac{1}{\tau^{-2} + \mathbf{1}^\top D^{-1} \mathbf{1}} \mathbf{1}^\top D^{-1}.$$

Equal loading  $\Rightarrow$  relative weights  $\propto D^{-1}$ ; correlation mainly slows learning.



# Estimation recipes

Binary (probabilities): logistic GLM on evaluation dates for intercept/responsiveness.

Gaussian (continuous): bias = mean residual; precision = inverse residual variance.

## Notation (for audience reference)

| Symbol     | Meaning                                                                |
|------------|------------------------------------------------------------------------|
| $N$        | number of experts                                                      |
| $\lambda$  | public prior; $\text{logit}(\lambda) = \log \frac{\lambda}{1-\lambda}$ |
| $p_L, p_H$ | low/high precision (hit rate or inverse variance)                      |
| $y_t^i$    | public report; $s_t^i$ private signal                                  |
| $\rho_t^i$ | reputation of expert $i$                                               |
